# Supplementary material for: Deterministic and dynamic synthesis of optical skyrmions through an ultrathin multimode fibre
Source: arXiv:2611.02549 source file (2026-11-02)
Supplement: Supplementary file 1 [file supplementary_information.tex]

\documentclass[11pt]{article}
\usepackage[a4paper,margin=2.2cm]{geometry}
\usepackage{graphicx,amsmath,amssymb,longtable,textcomp}
\usepackage[labelfont=bf,labelsep=period]{caption}
\renewcommand{\figurename}{Supplementary Figure}
\renewcommand{\tablename}{Supplementary Table}
\graphicspath{{SI/}}
\begin{document}
\begin{center}
{\Large\bfseries Supplementary Information}\\[1ex]
{\large Deterministic and dynamic synthesis of optical skyrmions through an ultrathin multimode fibre}\\[1ex]
R.~E.~Bautista Gonzalez, R.~Mouthaan, A.~McIntosh and K.~Dholakia
\end{center}
\bigskip
This document contains Supplementary Table~1, listing the components of the optical setup, and Supplementary Figs.~1--5, showing experimental results for anti-Bloch type, higher-order N\'eel type, higher-order Bloch type, bimeron-N\'eel type and bimeron-Bloch type optical skyrmions.

\section*{Supplementary Note 1: Optical setup components}
\begin{longtable}{p{2.5cm} p{9.6cm}}
\caption{\textbf{List of components used in the optical setup.}}
\label{tab:Setupcomponents}\\

\hline
Component & Specifications \\
\hline
\endfirsthead

\hline
Component & Specifications \\
\hline
\endhead

\hline
\endfoot

\hline
\endlastfoot

Laser & Coherent Sapphire CDRH SFNX 532-50 \\

Fibre Splitter & Thorlabs TN532R5F1 --- 1x2 Narrowband Fibre Optic Coupler, 532 ± 15 nm, 50:50 Split, FC/PC \\

Lens 1 & Thorlabs AC254-075-A-ML --- \(f = 75\) mm, Ø1" Achromatic Doublet \\

$\lambda$/2 wave plates & Thorlabs WPH10ME-532 --- Ø1" Mounted Polymer Zero-Order Half-Wave Plate \\

BS & Thorlabs CCM1-BS013/M --- 30 mm Cage Cube-Mounted Non-Polarising Beamsplitter, 50:50 (R:T), 400 - 700 nm \\

PBS & Thorlabs CCM1-PBS251/M --- 30 mm Cage Cube-Mounted Polarising Beamsplitter Cube, 420-680 nm \\

SLM 1 & Hamamatsu X10468-01 \\

SLM 2 & Meadowlark E19X12-400-700 \\

Lens 2 & Thorlabs AC254-150-A-ML --- \(f = 150\) mm, Ø1" Achromatic Doublet \\

Lens 3 & Thorlabs LB1901-A-ML --- \(f = 75\) mm, Ø1" Mounted N-BK7 Bi-Convex Lens \\

Objective & Olympus UPlanFL N Objective, 20$\times$0.5 NA \\

Fibre & Corning InfiniCor 300 graded-index multimode fibre (62.5/125 µm)\\

Lens 4 & Thorlabs LA1074-A --- \(f = 20\) mm, Ø1/2", N-BK7 Plano-Convex Lens\\

Lens 5 & Thorlabs AC254-200-A-ML --- \(f = 200\) mm, Ø1" Achromatic Doublet \\

Lens 6 & Thorlabs AC254-100-A-ML --- \(f = 100\) mm, Ø1" Achromatic Doublet \\

Camera 1 & FLIR Blackfly S BFS-U3-16S2M \\

Camera 2 & FLIR Blackfly S BFS-U3-16S2M \\

\end{longtable}

\section*{Supplementary Note 2: Other optical skyrmions}

\begin{figure}[p]
\centering
\includegraphics[width=0.6\linewidth]{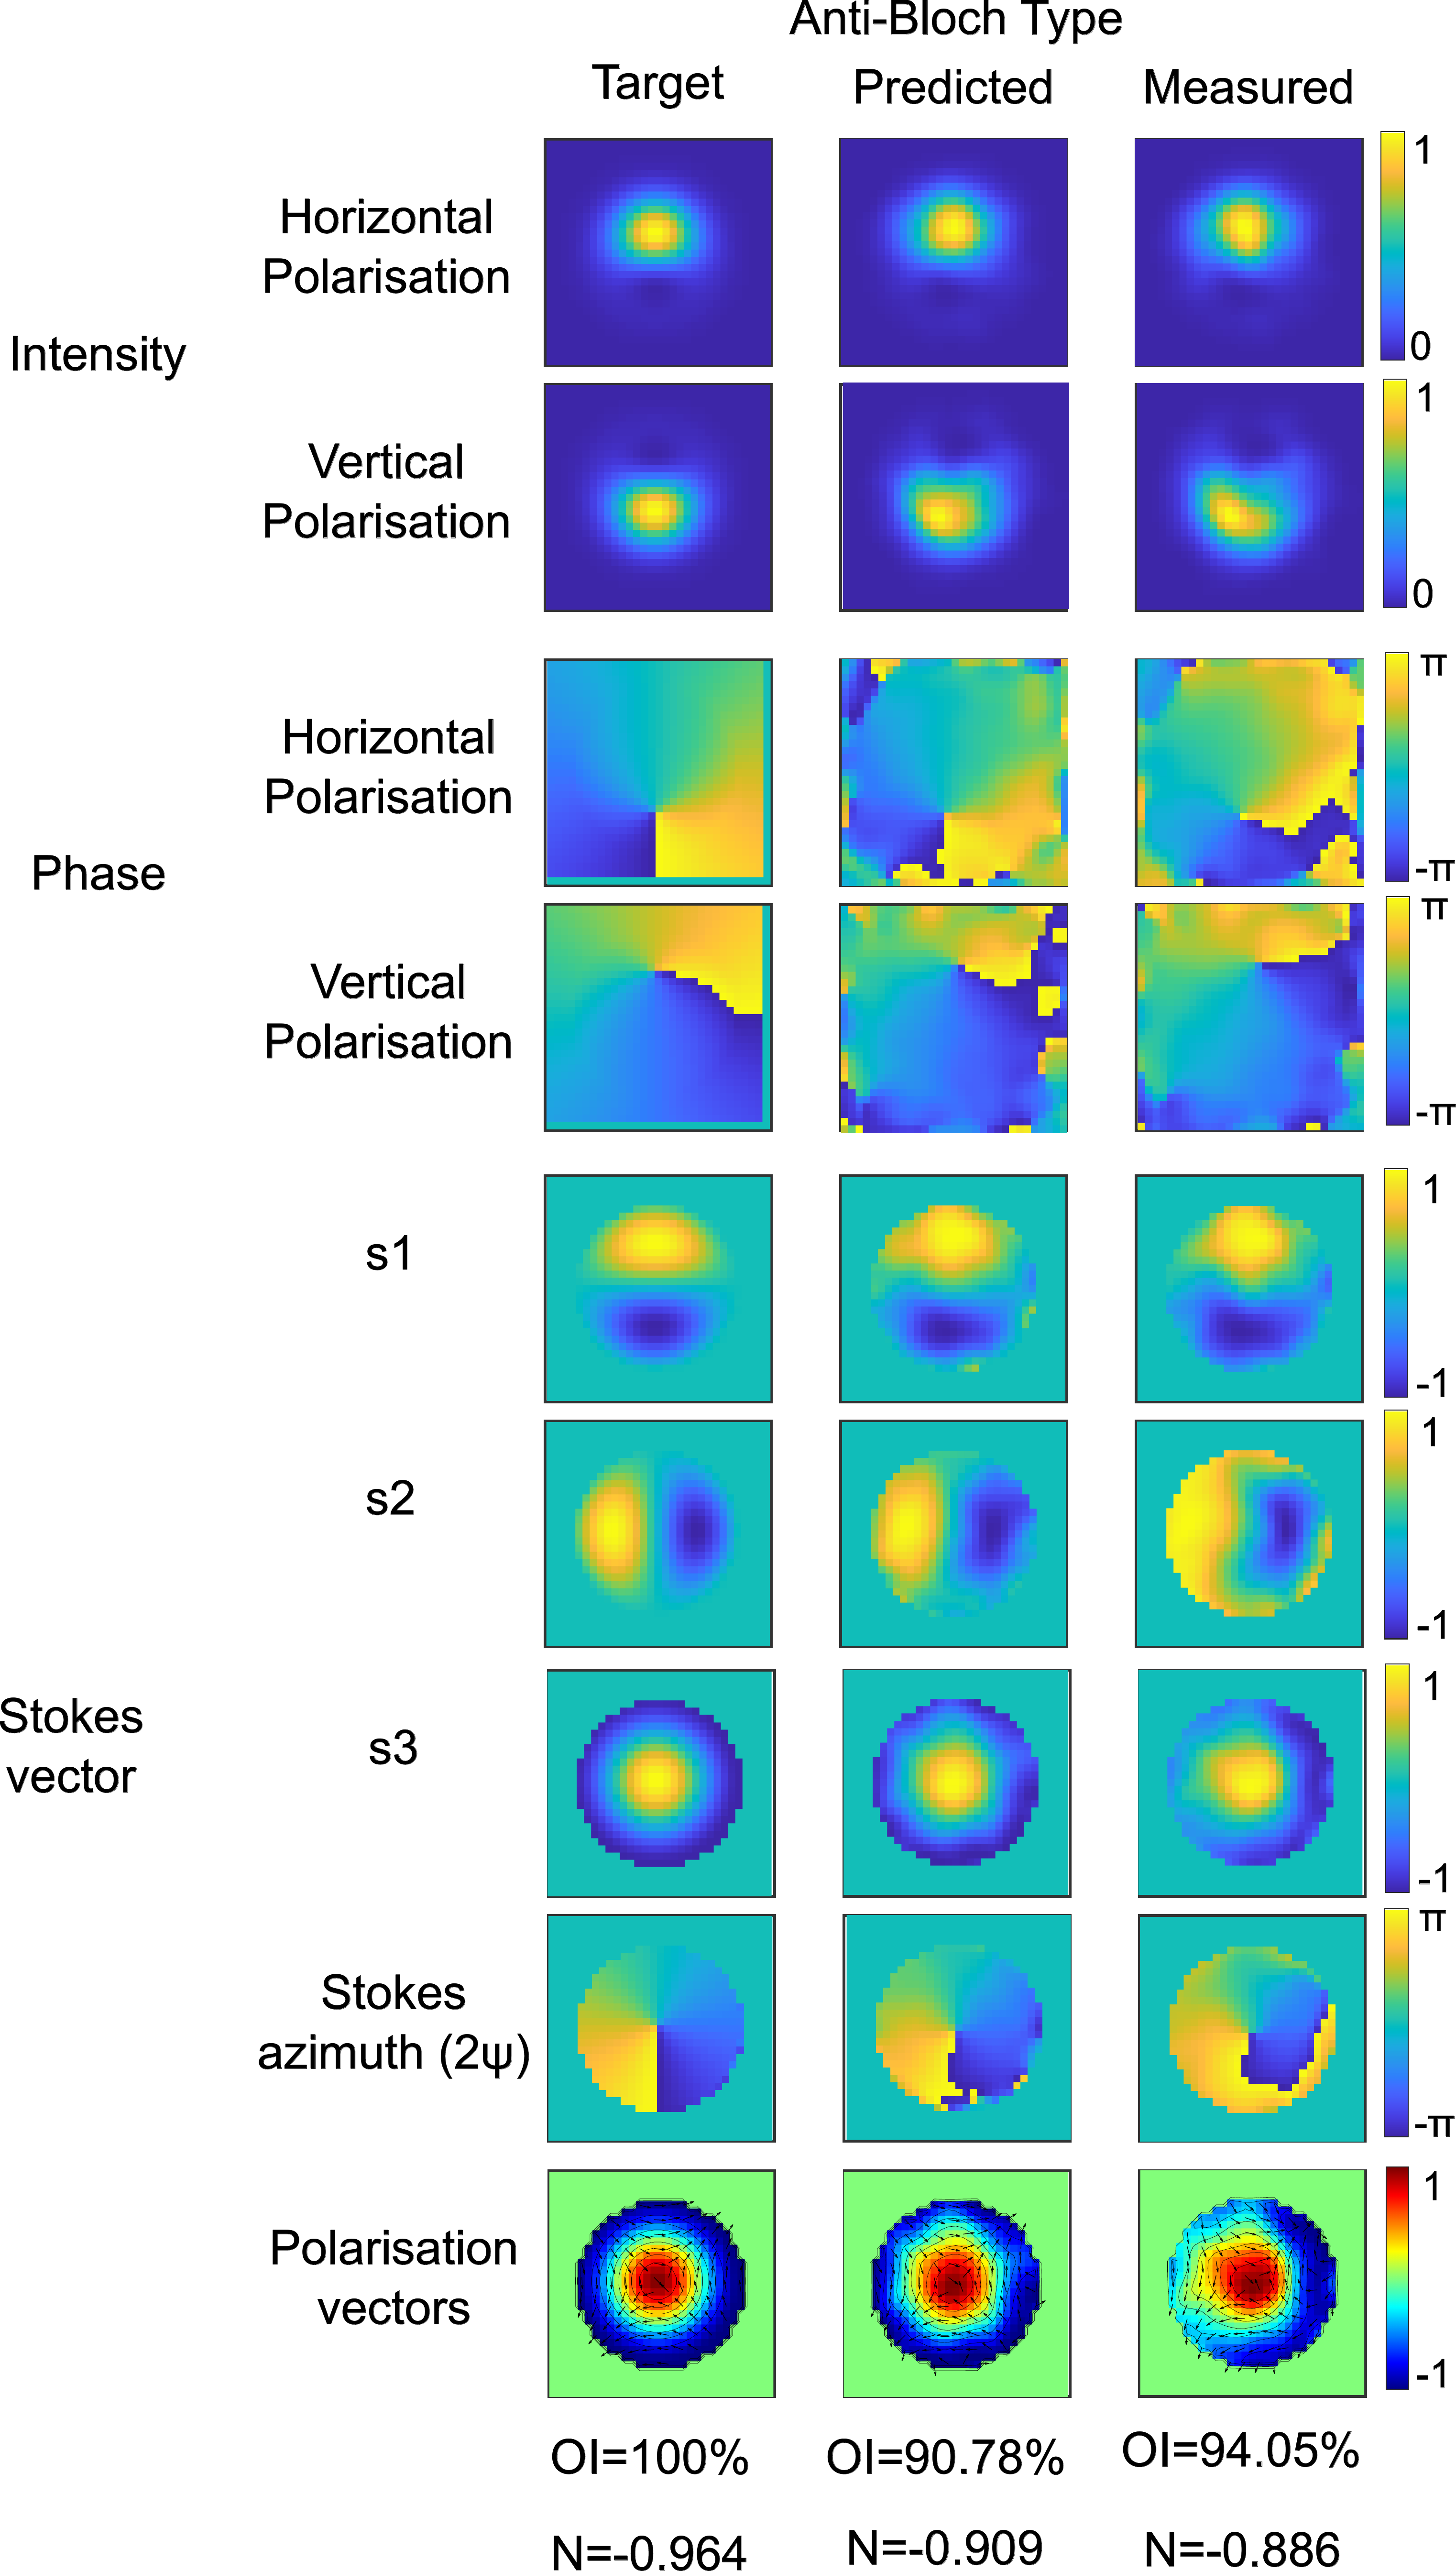}
\caption{\textbf{Generation and experimental characterisation of an anti-Bloch type optical skyrmion through dual-polarisation wavefront shaping.} The columns show the target field, the field predicted from the measured TM, and the experimentally measured field at the fibre output. The first four rows show the intensity and phase distributions of the horizontal and vertical polarisation components. The reconstructed complex fields are used to calculate the normalised Stokes parameters $s_1$, $s_2$, and $s_3$, together with the corresponding Stokes azimuth 2$\Psi$ and spatial polarisation-vector texture. The characteristic anti-Bloch polarisation texture is reproduced in both the predicted and measured fields. The overlap integral (OI) is $90.78\%$ for the predicted field with respect to the target field and $94.05\%$ for the measured field with respect to the predicted field. The corresponding skyrmion numbers are $N_{\mathrm{sk}}=-0.964$, $-0.909$, and $-0.886$ for the target, predicted, and measured fields, respectively, demonstrating preservation of the designed anti-Bloch-type topological structure.}
\label{fig:AntiBlochskyrmion}
\end{figure}

\begin{figure}[p]
\centering
\includegraphics[width=0.6\linewidth]{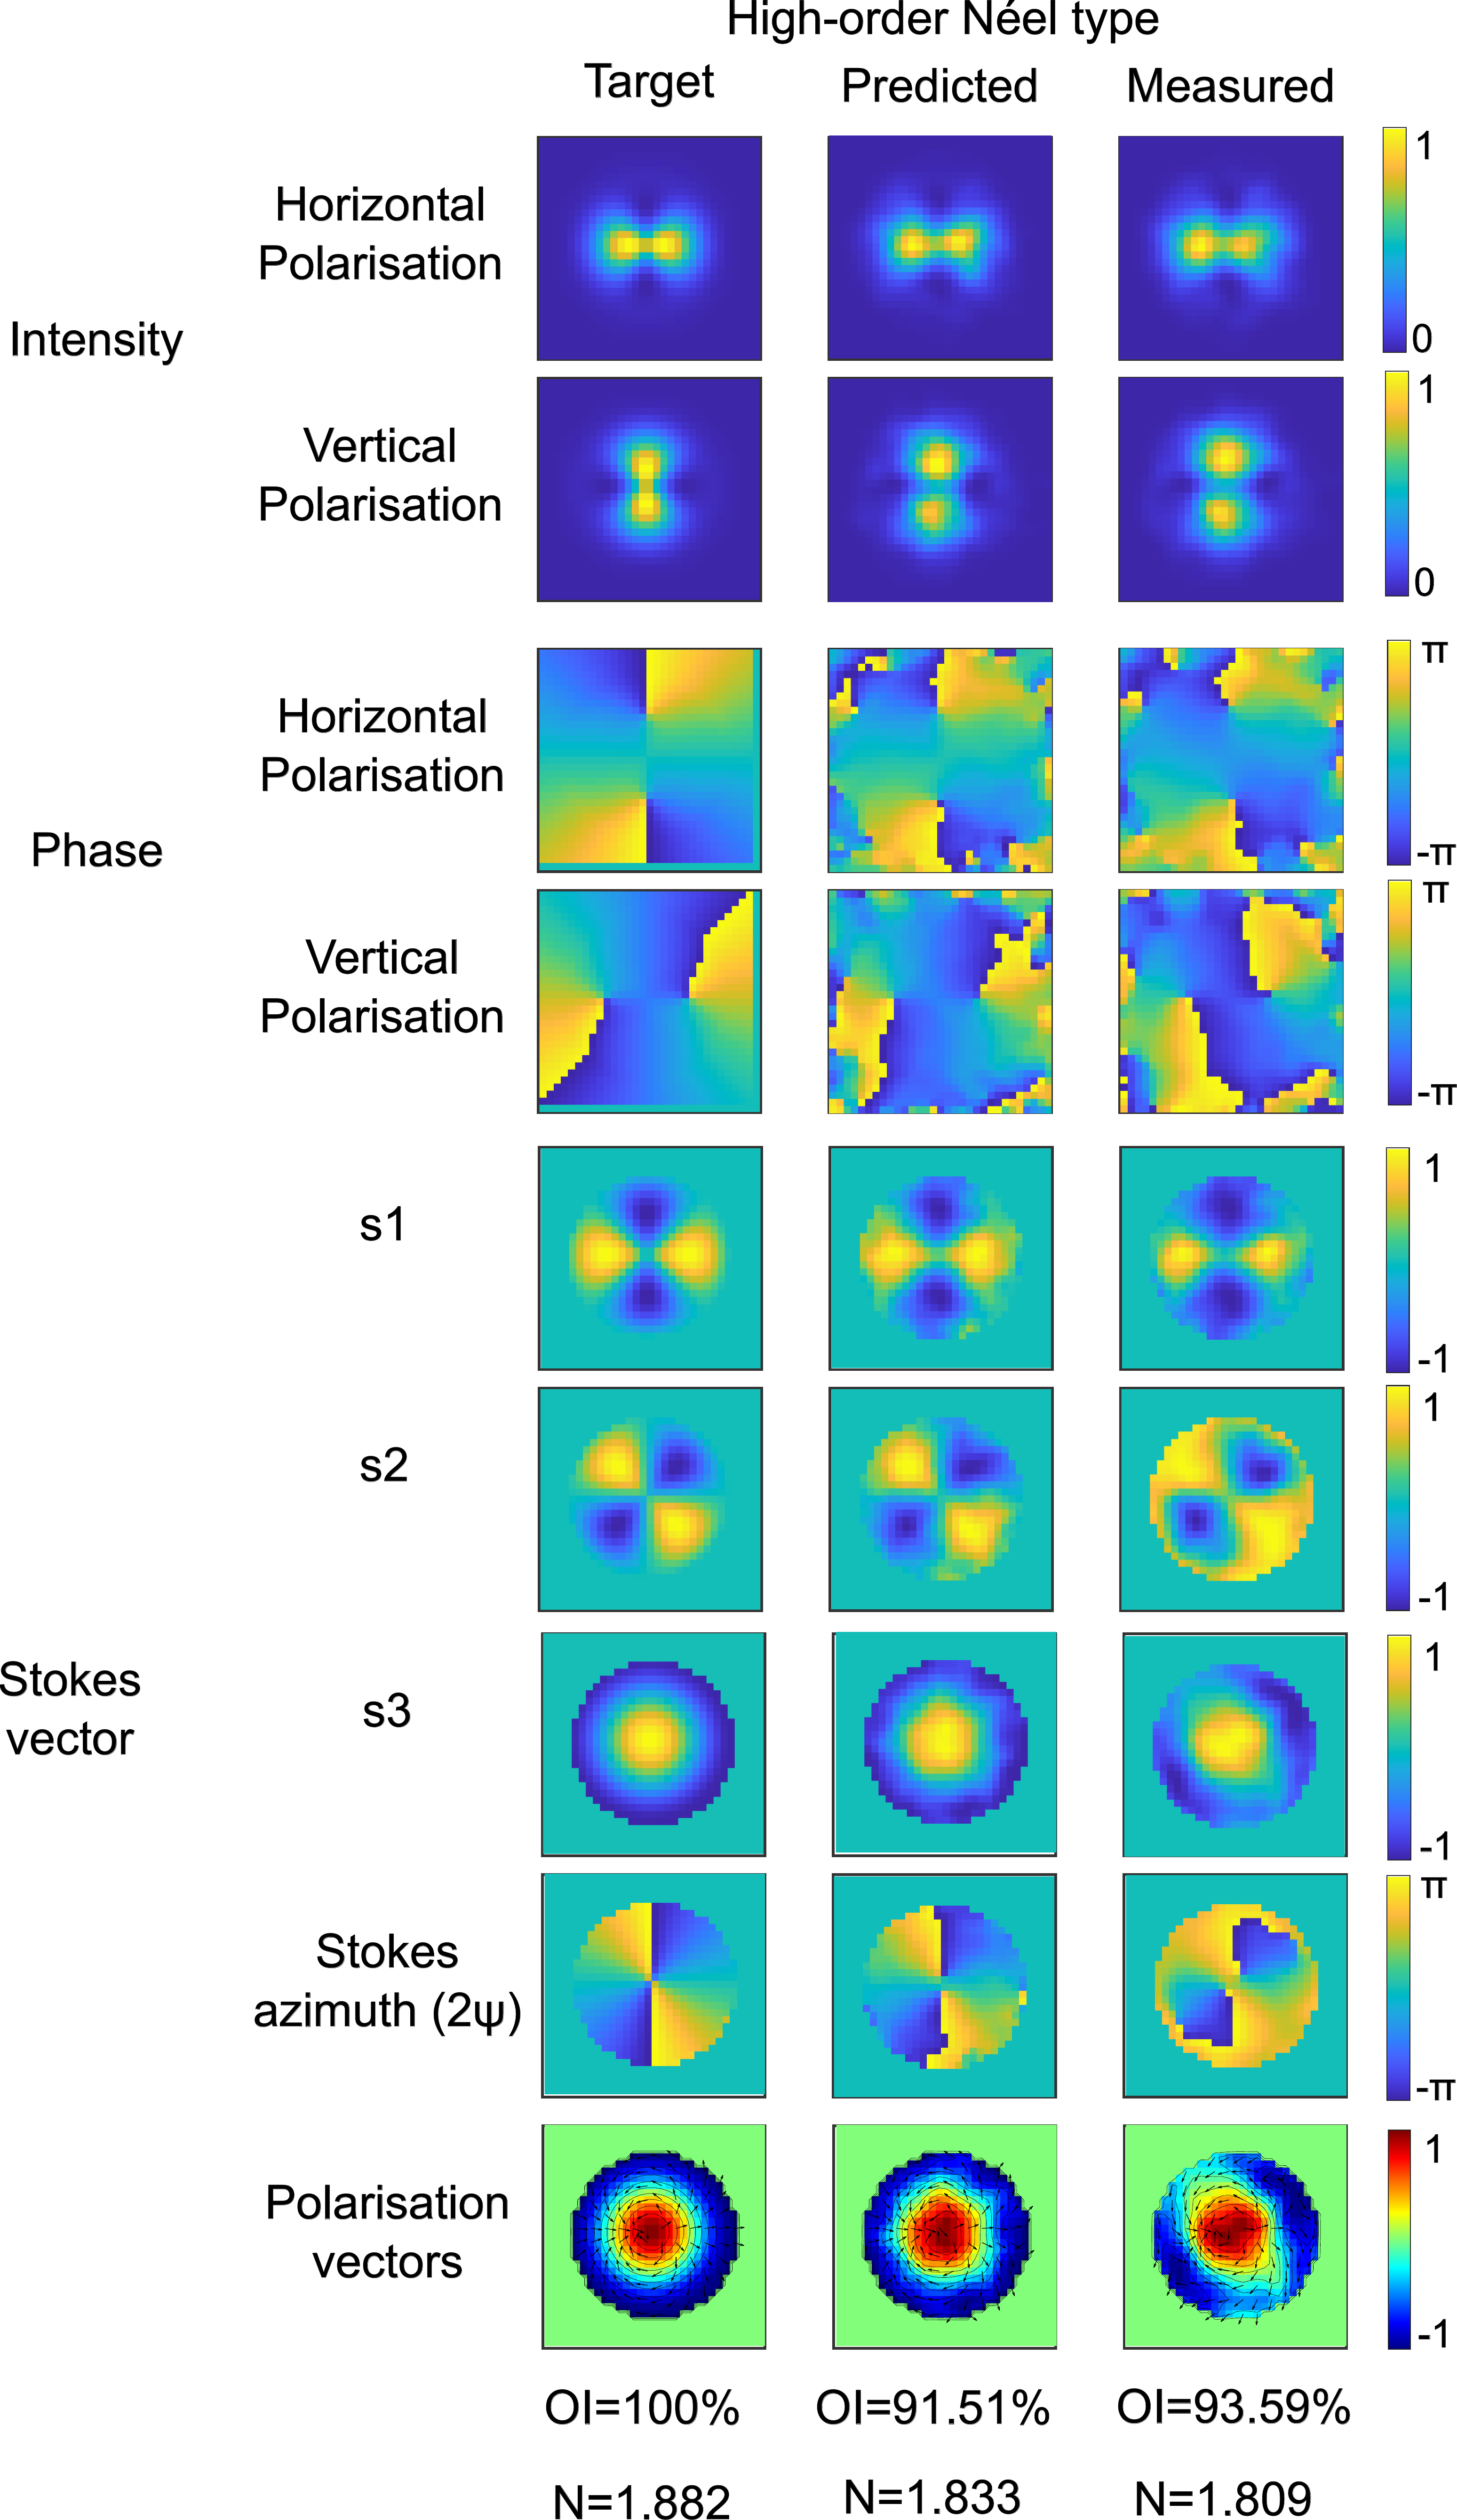}
\caption{\textbf{Generation and experimental characterisation of a high-order N\'eel type optical skyrmion through dual-polarisation wavefront shaping.} The columns show the target field, the field predicted from the measured TM, and the experimentally measured field at the fibre output. The first four rows show the intensity and phase distributions of the horizontal and vertical polarisation components. The reconstructed complex fields are used to calculate the normalised Stokes parameters $s_1$, $s_2$, and $s_3$, together with the corresponding Stokes azimuth 2$\Psi$ and spatial polarisation-vector texture. The higher-order N\'eel-type configuration exhibits the increased winding of the polarisation field associated with its higher topological order, which is reproduced in both the predicted and measured fields. The overlap integral (OI) is $91.51\%$ for the predicted field with respect to the target field and $93.59\%$ for the measured field with respect to the predicted field. The corresponding skyrmion numbers are $N_{\mathrm{sk}}=1.882$, $1.833$, and $1.809$ for the target, predicted, and measured fields, respectively, demonstrating preservation of the higher-order topological structure.}
\label{fig:HighNeelskyrmion}
\end{figure}

\begin{figure}[p]
\centering
\includegraphics[width=0.6\linewidth]{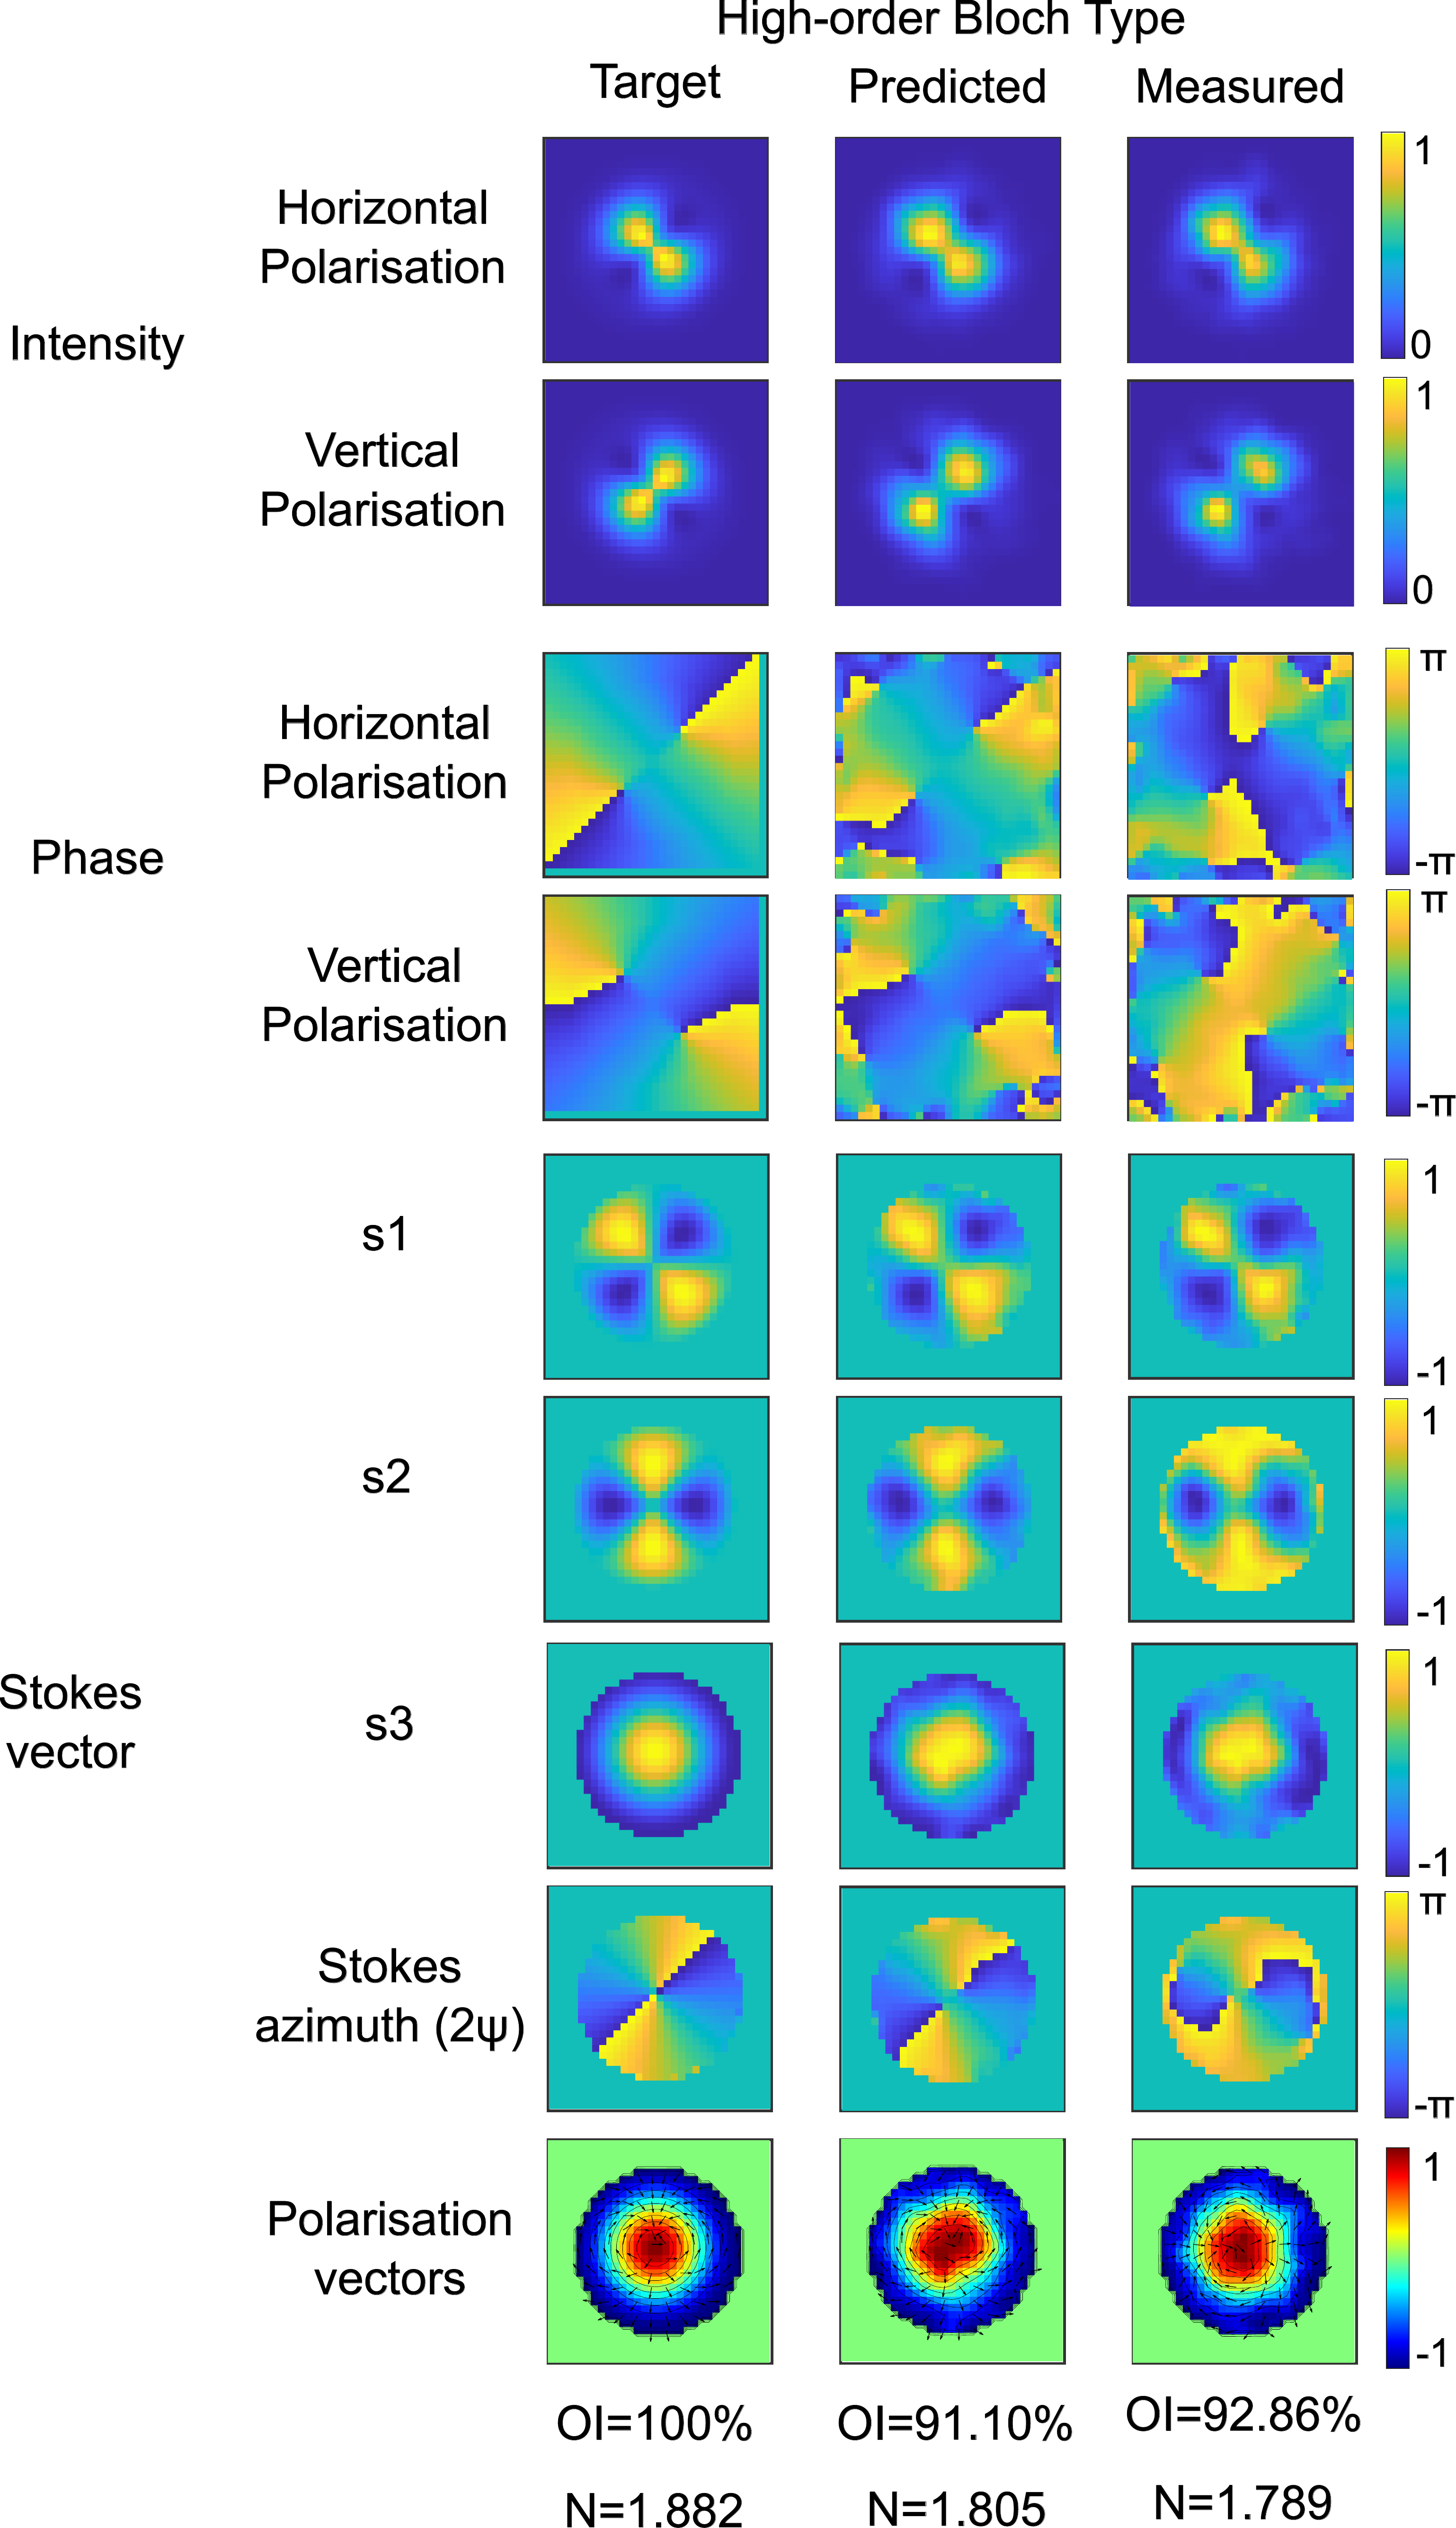}
\caption{\textbf{Generation and experimental characterisation of a high-order Bloch type optical skyrmion through dual-polarisation wavefront shaping.} The columns show the target field, the field predicted from the measured TM, and the experimentally measured field at the fibre output. The first four rows show the intensity and phase distributions of the horizontal and vertical polarisation components. The reconstructed complex fields are used to calculate the normalised Stokes parameters $s_1$, $s_2$, and $s_3$, together with the corresponding Stokes azimuth 2$\Psi$ and spatial polarisation-vector texture. The higher-order Bloch-type configuration exhibits the increased winding of the polarisation field associated with its higher topological order, which is reproduced in both the predicted and measured fields. The overlap integral (OI) is $91.10\%$ for the predicted field with respect to the target field and $92.86\%$ for the measured field with respect to the predicted field. The corresponding skyrmion numbers are $N_{\mathrm{sk}}=1.882$, $1.805$, and $1.789$ for the target, predicted, and measured fields, respectively, demonstrating preservation of the higher-order Bloch-type topological structure.}
\label{fig:HighBlochskyrmion}
\end{figure}

\begin{figure}[p]
\centering
\includegraphics[width=0.6\linewidth]{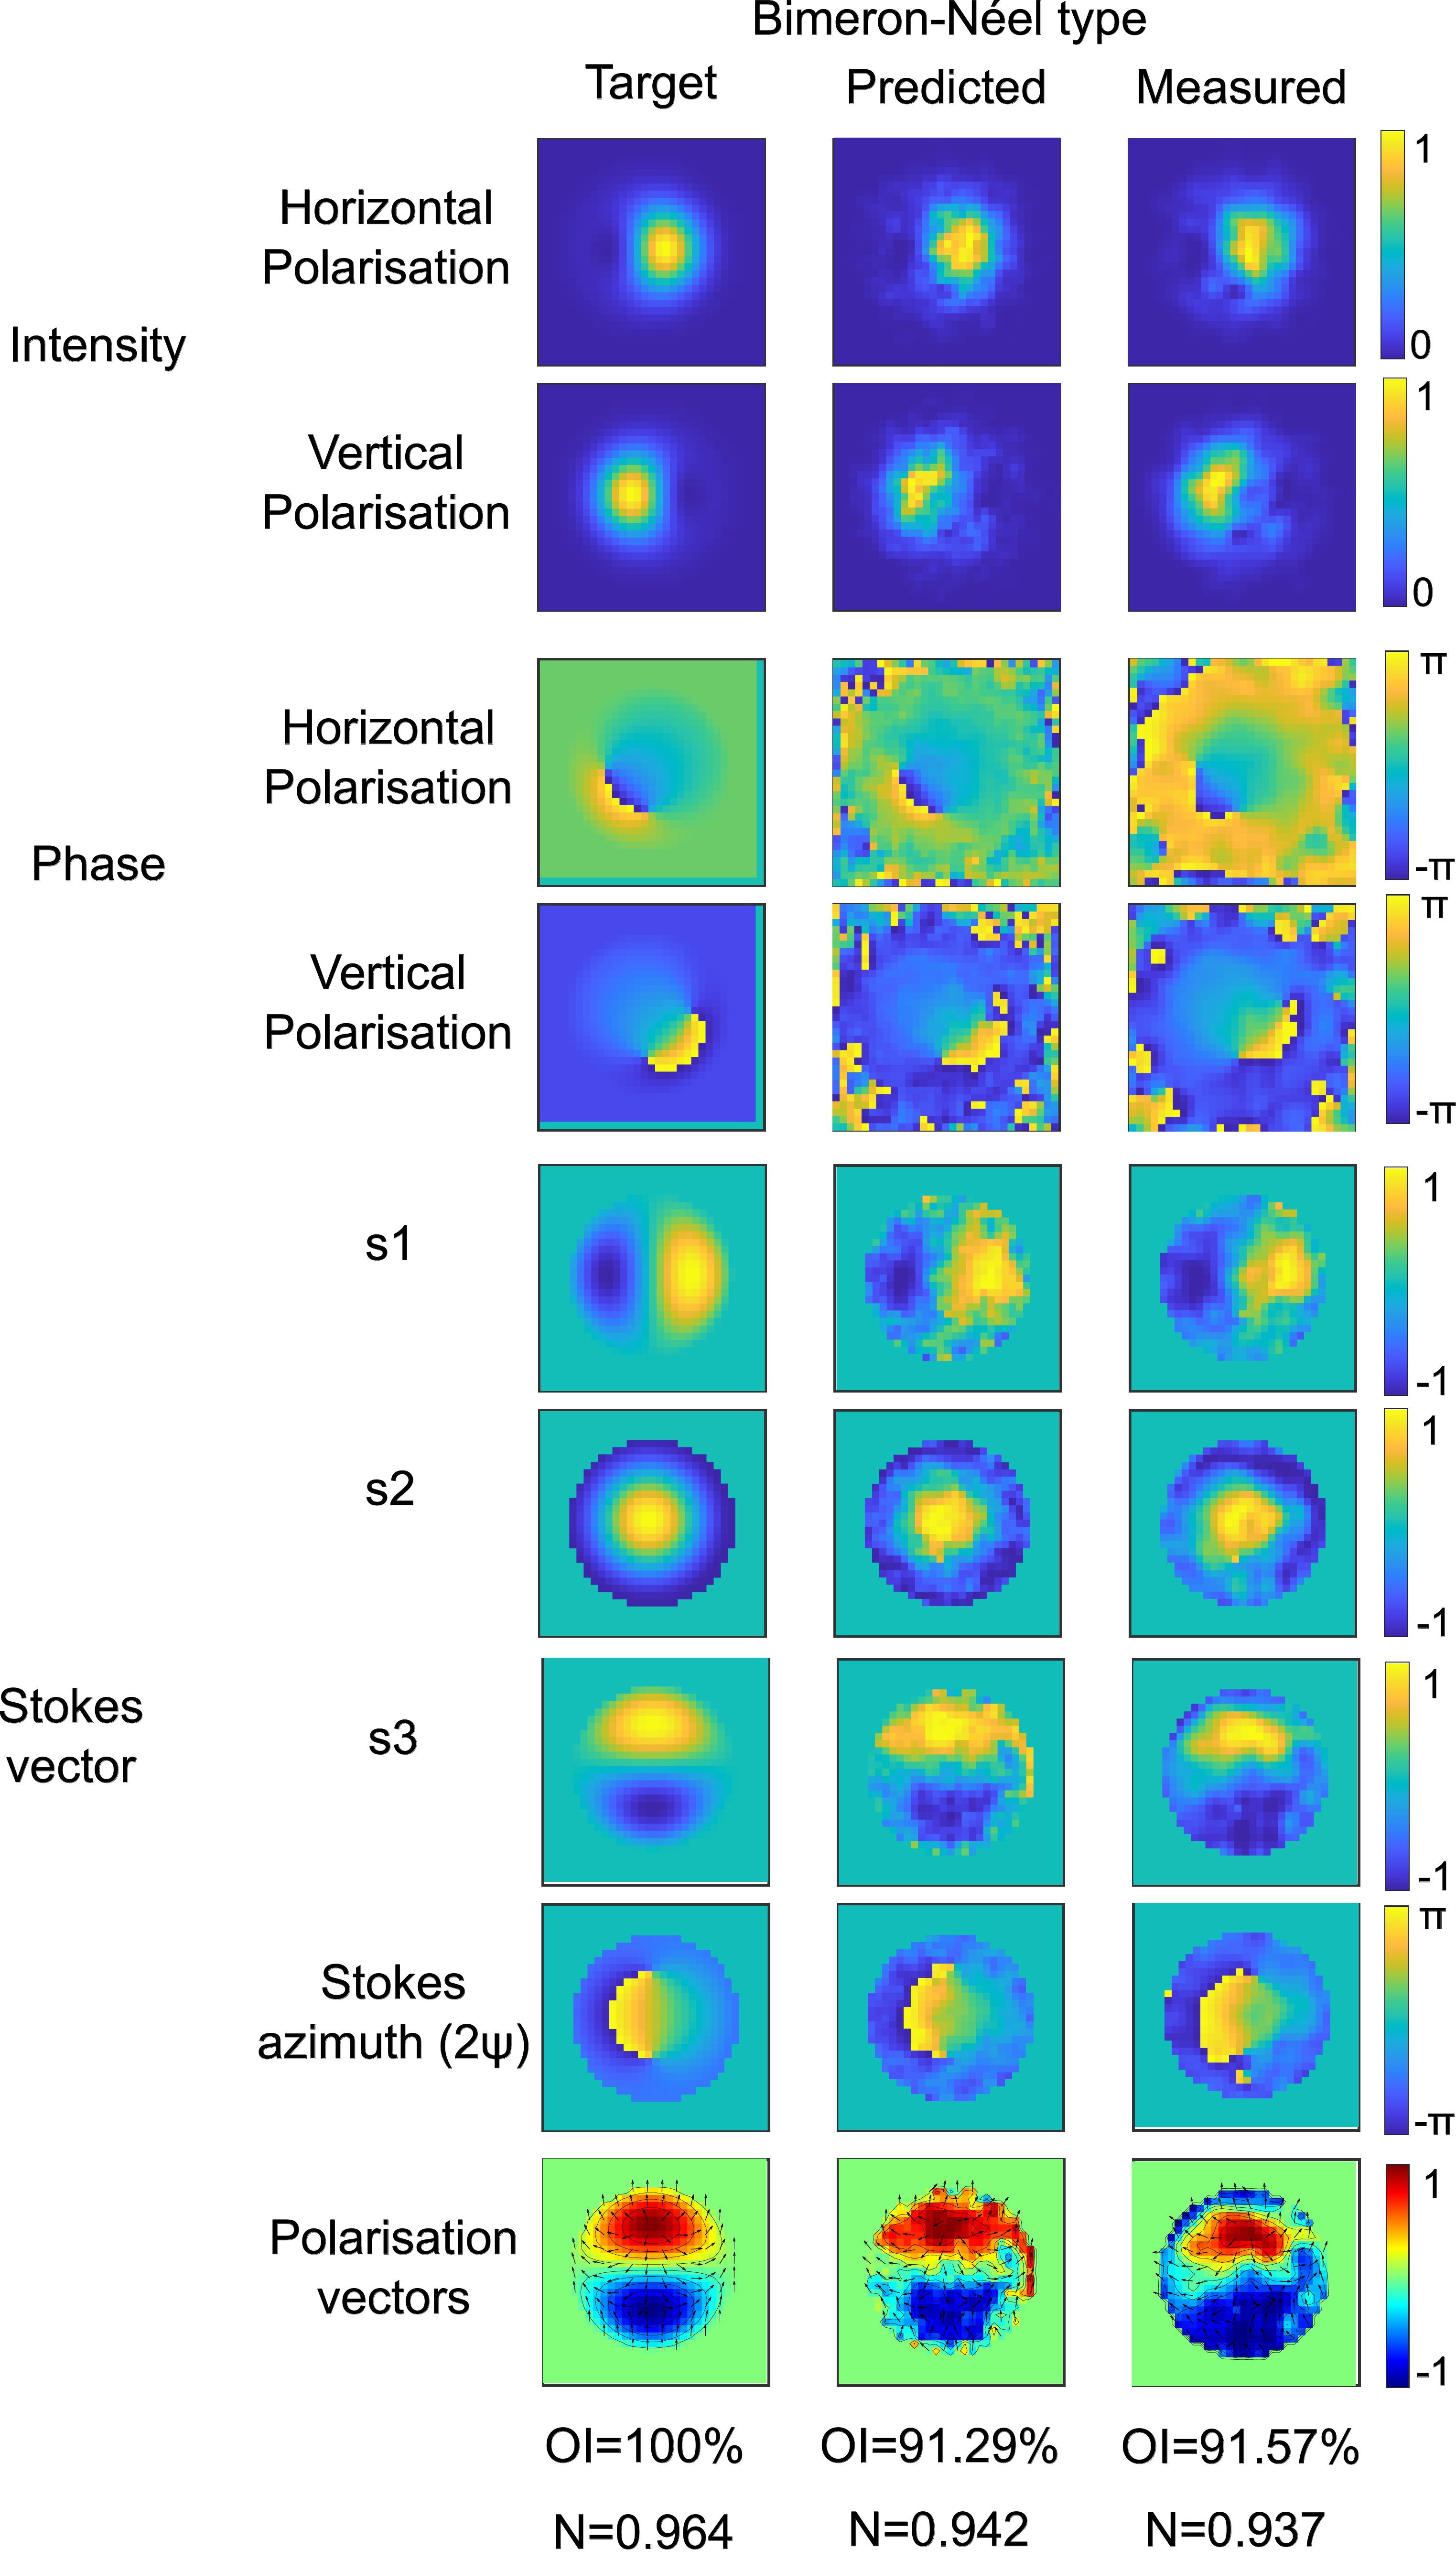}
\caption{\textbf{Generation and experimental characterisation of a N\'eel type optical bimeron through dual-polarisation wavefront shaping.} The columns show the target field, the field predicted from the measured TM, and the experimentally measured field at the fibre output. The first four rows show the intensity and phase distributions of the horizontal and vertical polarisation components. The reconstructed complex fields are used to calculate the normalised Stokes parameters $s_1$, $s_2$, and $s_3$, together with the corresponding Stokes azimuth 2$\Psi$ and spatial polarisation-vector texture. The characteristic N\'eel-type bimeron polarisation texture is reproduced in both the predicted and measured fields. The overlap integral (OI) is $91.29\%$ for the predicted field with respect to the target field and $91.57\%$ for the measured field with respect to the predicted field. The corresponding skyrmion numbers are $N_{\mathrm{sk}}=0.964$, $0.942$, and $0.937$ for the target, predicted, and measured fields, respectively, demonstrating preservation of the designed N\'eel-type bimeron structure.}
\label{fig:BimeronNeelskyrmion}
\end{figure}

\begin{figure}[p]
\centering
\includegraphics[width=0.6\linewidth]{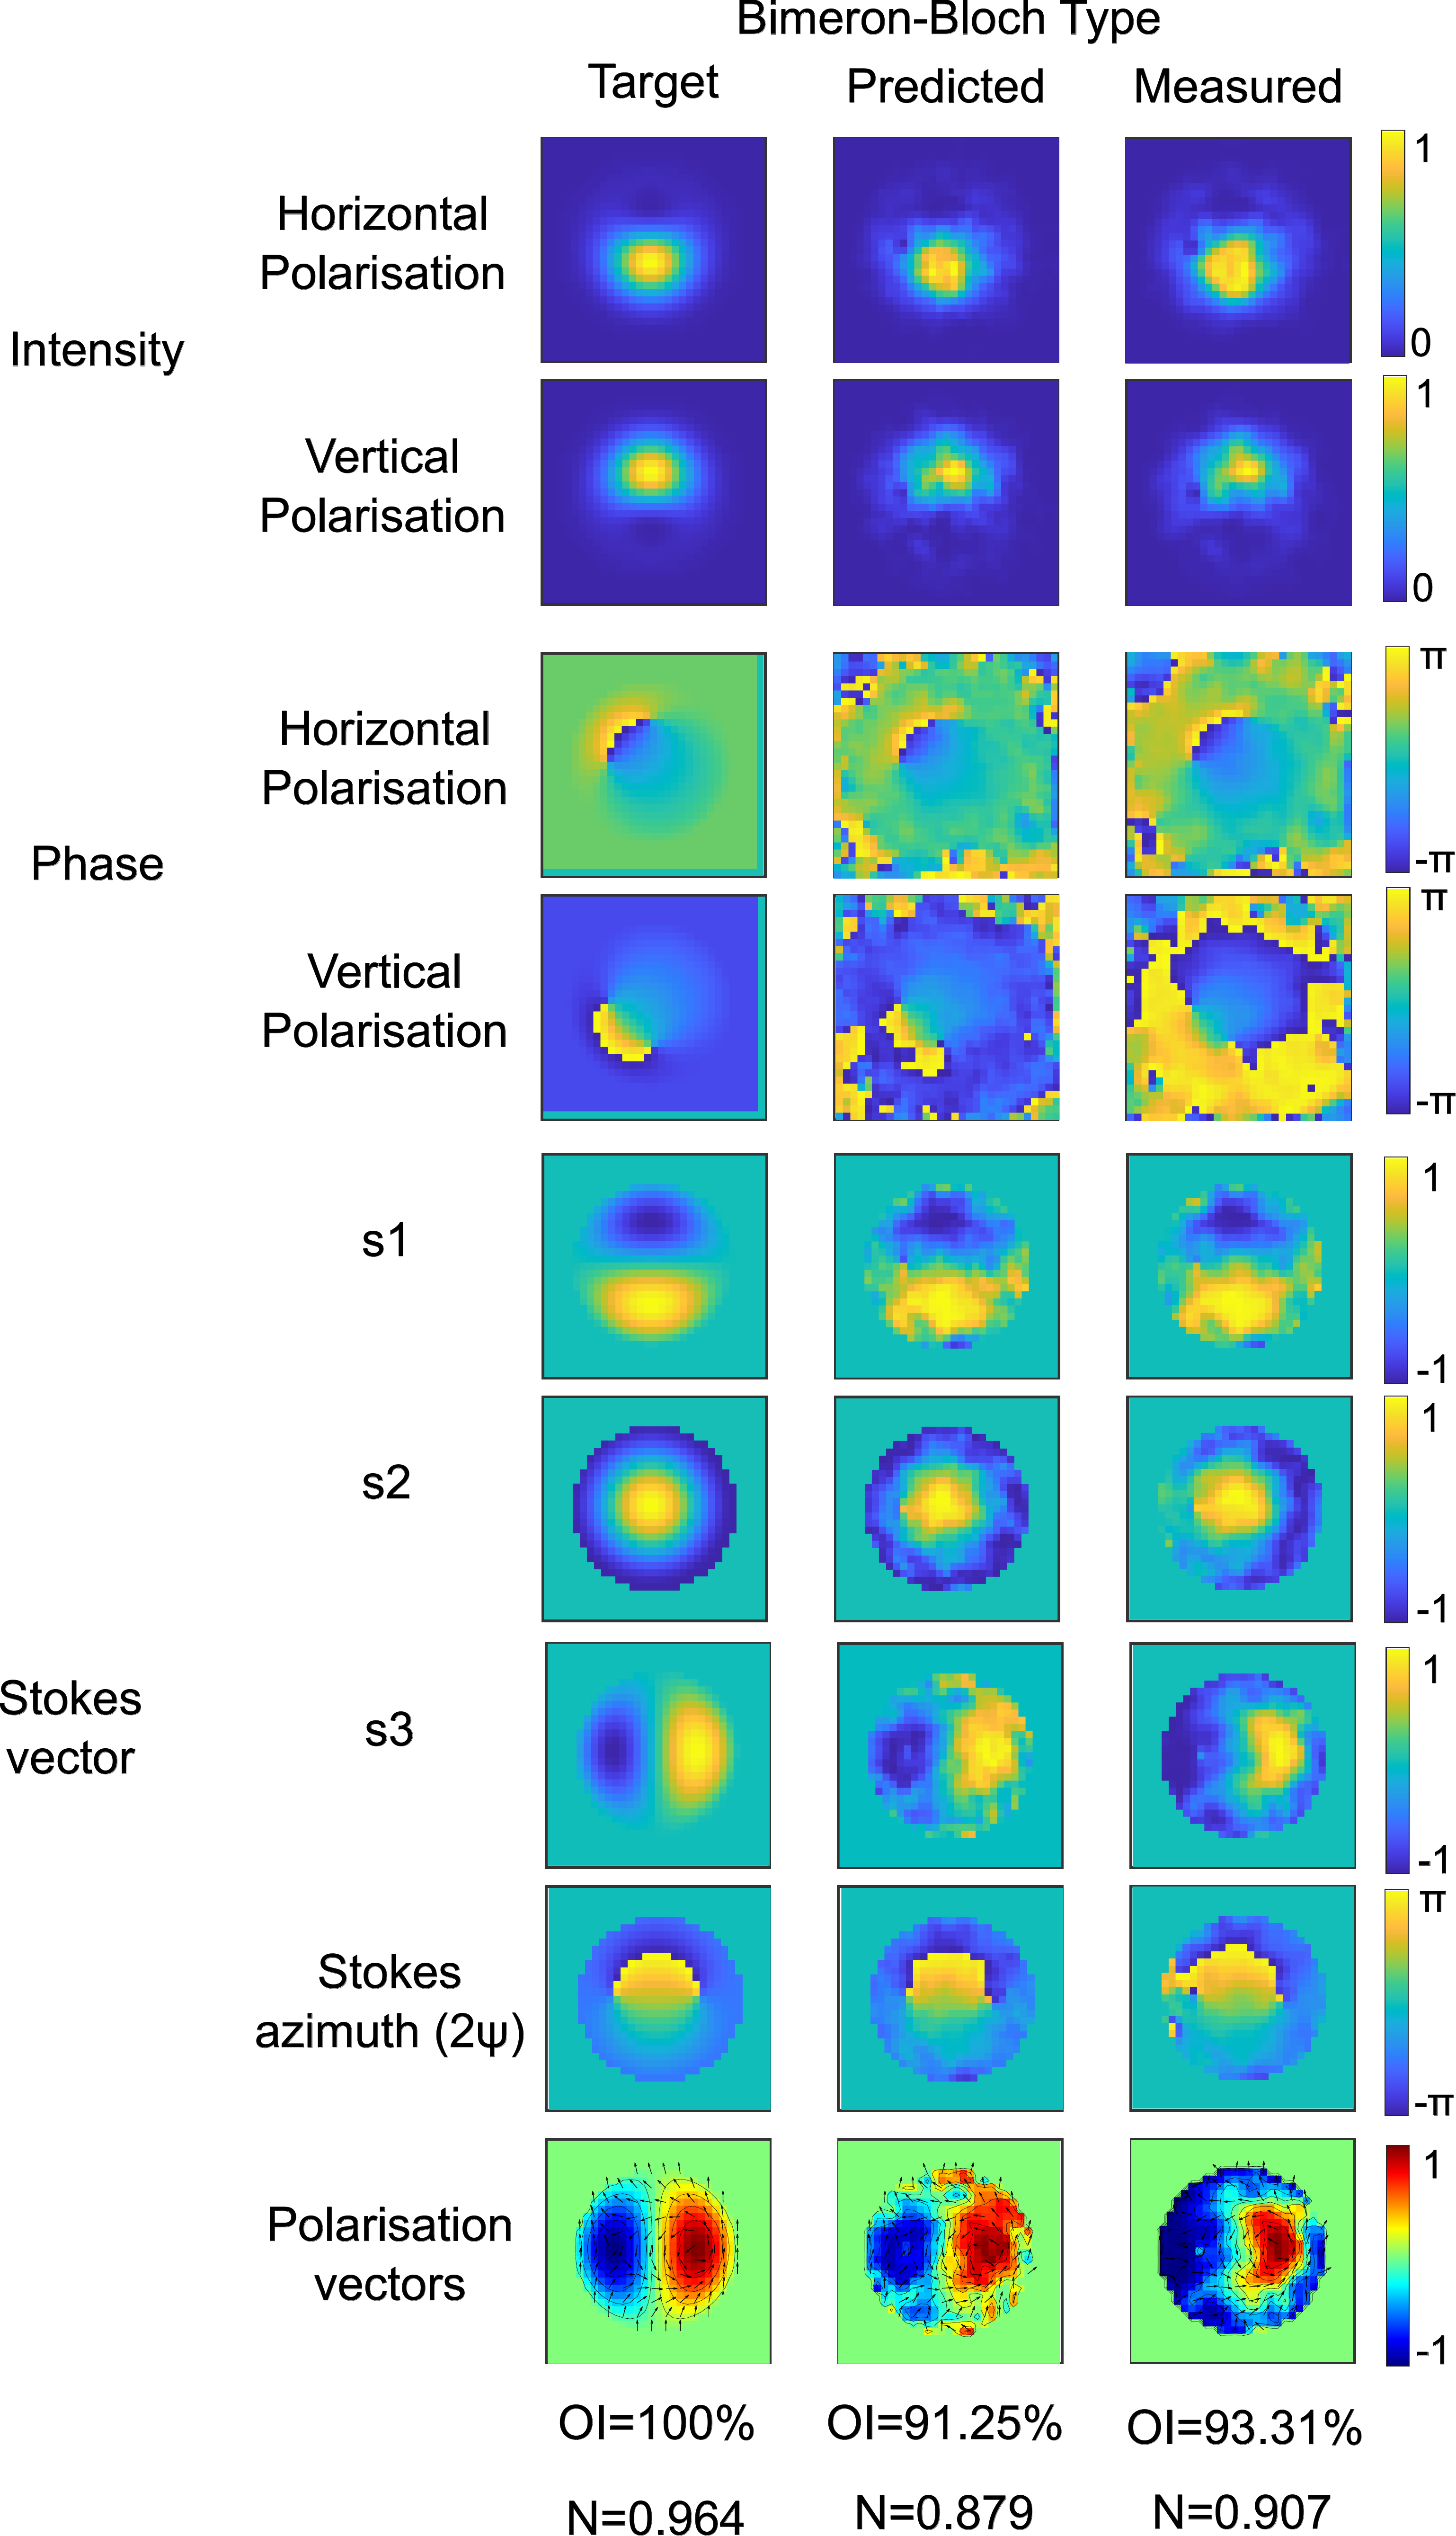}
\caption{\textbf{Generation and experimental characterisation of a Bloch type optical bimeron through dual-polarisation wavefront shaping.} The columns show the target field, the field predicted from the measured TM, and the experimentally measured field at the fibre output. The first four rows show the intensity and phase distributions of the horizontal and vertical polarisation components. The reconstructed complex fields are used to calculate the normalised Stokes parameters $s_1$, $s_2$, and $s_3$, together with the corresponding Stokes azimuth 2$\Psi$ and spatial polarisation-vector texture. The characteristic Bloch-type bimeron polarisation texture is reproduced in both the predicted and measured fields. The overlap integral (OI) is $91.25\%$ for the predicted field with respect to the target field and $93.31\%$ for the measured field with respect to the predicted field. The corresponding skyrmion numbers are $N_{\mathrm{sk}}=0.964$, $0.879$, and $0.907$ for the target, predicted, and measured fields, respectively, demonstrating preservation of the designed Bloch-type bimeron structure.}
\label{fig:BimeronBlochskyrmion}
\end{figure}

\end{document}
